# Supplementary material for: The first all-sky view of the Milky Way stellar halo with Gaia+2MASS RR Lyrae
Source: arXiv:1707.03833 source file (2017-11-02)
Supplement: Supplementary file 1 [file lnlike.tex]

\section{The likelihood of a distribution of stars} \label{app:lnlike}
Suppose that the expected  rate  function  for finding  a stars  in the infinitesimal observational volume $\te{d}S=\te{d}m\te{d}\Omega$ is expressed as 
\begin{equation}
\lambda=\lambda_c \tilde{\lambda},
\label{eq:rate}
\end{equation}
where  $\lambda_c$ is the rate  amplitude and $\tilde{\lambda}$ represents the normalised rate function.
Given  the rate function in Eq. \ref{eq:rate}, the  expected number of stars in a certain  position in the sky (l,b)  and  at a certain magnitude $m$  is Poisson distributed. Therefore, the probability to  find  $x$ stars in  at certain position  is 
\begin{equation}
P(x)=e^{-\lambda} \frac{\lambda^x}{x!}.
\label{eq:poio}
\end{equation} 
Suppose that we have   $N_\textrm{s}$ stars  distributed over the sky  and over an  interval of apparent magnitude. Let use divide  all the volume covered by  the stars in infinitesimal intervals of volume $\te{d}S=\te{d} \Omega \te{d}m$. We will obtain $N_\textrm{s}$ infinitesimal bins containing one star and $N_\textrm{n}$ empty bins. Using Eq. \ref{eq:poio}, the likelihood of our data is 
\begin{equation}
\mathcal{L}(\text{0 in }N_\text{n}; \text{1 in }N_{\text{tot}})= \prod^{N_\text{n}}_j  e^{-\lambda_i} \cdot \prod^{N_\text{s}}_i \lambda_i e^{-\lambda_i}
\label{eq:poi}
\end{equation}
and the logarithmic likelihood is
\begin{equation}
\ln \mathcal{L}=   \sum^{N_\text{s}}_i \ln \lambda_i - \left(\sum^{N_\text{s}}_i \lambda_i + \sum^{N_\text{n}}_j \lambda_j \right).
\label{eq:poilog}
\end{equation}
The last two terms of Eq. \ref{eq:poilog} indicate a summation of $\lambda$ over all the infinitesimal bins with one or zero objects Therefore,  the two terms inside the parentheses  represent the definition of the integral over the total volume $S$ and Eq. \ref{eq:poilog} becomes 
\begin{equation}
\ln\mathcal{L}= \sum^{N_\text{s}}_i \ln \lambda_i - \Lambda,
\label{eq:poilog2}
\end{equation}
where 
\begin{equation}
\Lambda= \int_S \lambda \te{d}S = \lambda_c \int_S \tilde{\lambda} \te{d}S = \lambda_c  \te{V}_c
\label{eq:Lambda}
\end{equation}
is the expected number of stars in the whole volume $S$ and $\te{V}_c$ is the \vir{normalisation} integral.
Using Eq. \ref{eq:Lambda} we can write the rate amplitude as $\lambda_c=\Lambda \te{V}^{-1}_c$
and the logarithmic likelihood  becomes 
\begin{equation}
\ln\mathcal{L}=   \sum^{N_\text{s}}_i \ln \frac{\tilde{\lambda}}{\text{V}_c} - \Lambda +  N_\te{s} \ln \Lambda.
\label{eq:poilog3}
\end{equation}
If we are not interested on the normalisation scale ($\lambda_c$ or $\Lambda$), we can marginalise 
Eq. \ref{eq:poilog3} over $\Lambda$ using using a proper wide  prior (see e.g.  \citealt{bovymethod}). 
Therefore, up to a constant,  the logarithmic  likelihood becomes
\begin{equation}
\ln\mathcal{L}=   \sum^{N_\text{s}}_i \ln \frac{\tilde{\lambda}}{\text{V}_c}.
\label{eq:poilog4}
\end{equation}

The logarithmic likelihoods in Eq. \ref{eq:poilog4} has been obtained making the implicit assumption that  all the stars have the same absolute magnitude $M$. If absolute magnitude of the stars follows a certain distribution $\Phi(M)$, Eq. \ref{eq:poilog4} is still valid, but   the  normalised rate function $\tilde{\lambda}$ and the normalisation integral $\text{V}_c$ (Eq. \ref{eq:Lambda})  must be considered marginalised over $M$.

\subsection{Double population model} \label{app:multicomp}
The  logarithmic likelihood  in Eq.  \ref{eq:poilog3} and Eq. \ref{eq:poilog4} are valid  if all the stars in the sample come from a population with a single rate  function  $\lambda$. Suppose to have  a distribution of $N_\te{s}=N_\te{h}+N_\te{d}$ stars  where  $N_\te{h}$ stars belong to a population with  a rate function 
$\lambda_\te{h}=\lambda_{c\te{h}} \tilde{\lambda}_\te{h}$ and the other $N_\te{d}$ come from a population  with rate function $\lambda_\te{d}=\lambda_{c\te{d}} \tilde{\lambda}_\te{d}$, both defined as in Eq. \ref{eq:rate}.  
If stars belonging to the two different populations can be distinguished,  the  likelihood of the data is just the  product of the individual likelihoods expressed in Eq. \ref{eq:poi}, as a  consequence the final logarithmic likelihood  is the sum of the individual logarithmic likelihood expressed, up to a constant, in  Eq. \ref{eq:poilog4}:
\begin{equation}
\ln\mathcal{L}=\sum^{N_\te{h}}_i  \ln \frac{\tilde{\lambda}_\te{h}}{\te{V}_\te{h}} +  \sum^{N_\te{h}}_j  \ln \frac{\tilde{\lambda}_\te{d}}{\te{V}_\te{d}}.
\label{eq:lnknow}
\end{equation}

If it is not possible to distinguish  the stars  between the two  populations,  we  can define a global  rate function, $\lambda$, for finding  a stars (whatever population it belongs)  in a certain position of the observational space. In this case, $\lambda$  is  given by the sum of the  single rate functions:
\begin{equation}
\lambda=  \frac{\Lambda_\te{h}}{\te{V}_\te{h}}  \tilde{\lambda}_\te{h}  +  \frac{\Lambda_\te{d}}{\te{V}_\te{d}}  \tilde{\lambda}_\te{d},
\label{eq:double}
\end{equation}
where we have used Eq. \ref{eq:Lambda} to replace the rate amplitudes  $\lambda_{c\te{h}}$ and $\lambda_{c\te{d}}$  with the ratios between the expected numbers of stars in the whole volume $S$ ($\Lambda_\te{h}$, $\Lambda_\te{d}$)  and the normalisation integrals ($\te{V}_\te{h}, \te{V}_\te{d}$). Moreover,
we can define the  total expected number of stars $\Lambda=\int \lambda \te{d}S$ in the volume $S$ as
\begin{equation}
\Lambda=\Lambda_\te{h} + \Lambda_\te{d}
\label{eq:sumLambda}
\end{equation}
and the disc-to-total stellar ratio as
\begin{equation}
f=\frac{\Lambda_\te{d}}{\Lambda}.
\label{eq:ffracd}
\end{equation}
Using Eq. \ref{eq:sumLambda} and Eq. \ref{eq:ffracd} the rate function (Eq. \ref{eq:double}) becomes
\begin{equation}
\lambda= \Lambda \left( \frac{1-f}{\te{V}_\te{h}}  \tilde{\lambda}_\te{h} +   \frac{f}{\te{V}_\te{d}}  \tilde{\lambda}_\te{d} \right).
\label{eq:double2}
\end{equation}
Using  Eq. \ref{eq:double2} in  Eq. \ref{eq:poilog2} and marginalising over $\Lambda$ we obtain, up to a constant, the final logarithmic likelihood 
\begin{equation}
\ln\mathcal{L}=   \sum^{N_\text{s}}_i \ln \left( \frac{1-f}{\te{V}_\te{h}}  \tilde{\lambda}_\te{h} +   \frac{f}{\te{V}_\te{d}}  \tilde{\lambda}_\te{d} \right).
\label{eq:lndobule}
\end{equation}

As in the previous case the normalised rate functions and the normalisation integrals  of both halo and disc stars are implicitly assumed to be marginalised over their own distributions of the absolute magnitude.
